# Supplementary material for: Personalized Federated Learning of Driver Prediction Models for Autonomous Driving
Source: arXiv:2112.00956 source file (2021-12-02)
Supplement: Supplementary file 1 [file IOT_TPU.tex]

\begin{figure}
    \centering
    \includegraphics[width=0.99\columnwidth]{pics/IoT_sensor.pdf} % first figure itself
    \caption{(Left) Environmental sensor on the Google Edge Tensor Processing Unit (TPU) and example stochastic timeseries measurements (right). Our experiments in Sec. \ref{sec:experiments} illustrate how \name can compress these sensory measurements for anomaly detection using a neural network task module.}
    \label{fig:IoT}
\end{figure}
