# Supplementary material for: Personalized Federated Learning of Driver Prediction Models for Autonomous Driving
Source: arXiv:2112.00956 source file (2021-12-02)
Supplement: Supplementary file 2 [file LQR.tex]

% smaller
%%%%%%%%%%%%%%%%%%%%%%%%%%%%%%%%%%%%%%%%
\begin{figure}
    \centering
    \subfloat{
    \includegraphics[width=0.49\columnwidth]{pics/LQR_results/weighted_plots_codesign_inference_m_2_n_4/compare_norm_task_loss_per_step.pdf} % first figure itself
    \label{fig:LQR_2D_task_loss}
    }
    \subfloat {
        \includegraphics[width=0.49\columnwidth]{pics/LQR_results/weighted_plots_codesign_inference_m_2_n_4/compare_recon_loss_vec_per_step.pdf} % first figure itself
    \label{fig:LQR_2D_recon_loss}
    }
    \caption{\textbf{Illustrative example of the benefits of task-aware compression.} (Left, a) Even when the encoder, decoder, and task module are matrices with a bottleneck $z$, optimizing for task loss yields better task accuracy for smaller $z$, which we can analytically prove for the simplified linear setting. (Right, b) However, there is a tradeoff with reconstruction loss, prompting our use of a weighted reconstruction and task loss.}
    \label{fig:LQR_simulation}
\end{figure}
