# Supplementary material for: Personalized Federated Learning of Driver Prediction Models for Autonomous Driving
Source: arXiv:2112.00956 source file (2021-12-02)
Supplement: Supplementary file 3 [file MNIST_recon_unweighted.tex]

% smaller
%%%%%%%%%%%%%%%%%%%%%%%%%%%%%%%%%%%%%%%%
\begin{figure}
    \centering
    \includegraphics[width=1.0\columnwidth]{pics/reconstructed_MNIST/unweighted/task_recon_zdim_4_reconstruction_70.png}
    \caption{\textbf{MNIST classification \textit{without} reconstruction loss}: 
    Our general co-design framework also allows us to create highly-compressible representations that are purely optimized for a machine's task loss with reconstruction weight $\lambda=0.0$ (Eq. \ref{eq:weighted_loss}). Though we have a heavily-compressed representation with a size of $\zbottleneck=4$, decoded images $\xhat$ (bottom row) are \textit{not} human-interpretable and don't resemble original images $x$ (top row), unlike the scenario of Fig. \ref{fig:mars_recon_weighted}. This motivates our addition of a regularization term with reconstruction weight $\lambda > 0$ to develop representations that are highly-compressible, but yield interpretable decoded samples $\xhat$ as in Fig. \ref{fig:mars_recon_weighted}.}
    \label{fig:mars_recon_unweighted}
\end{figure}
