# Supplementary material for: Personalized Federated Learning of Driver Prediction Models for Autonomous Driving
Source: arXiv:2112.00956 source file (2021-12-02)
Supplement: Supplementary file 4 [file MNIST_recon_unweighted_2.tex]

% smaller
%%%%%%%%%%%%%%%%%%%%%%%%%%%%%%%%%%%%%%%%
\begin{figure}
    \centering
    \includegraphics[width=1.0\columnwidth]{pics/reconstructed_MNIST/unweighted/task_recon_zdim_4_reconstruction_60.png}
    \caption{\textbf{MNIST \textit{without} reconstruction loss}: 
    A further example of how optimizing for purely a machine's task loss, without reconstruction weight $\lambda$, yields highly-compressible, but uninterpretable decoded images $\xhat$. This example mirrors Fig. \ref{fig:mars_recon_unweighted}, but for another set of data.}
    \label{fig:mars_recon_unweighted_2}
\end{figure}
