# Supplementary material for: Personalized Federated Learning of Driver Prediction Models for Autonomous Driving
Source: arXiv:2112.00956 source file (2021-12-02)
Supplement: Supplementary file 5 [file MNIST_recon_weighted.tex]

% smaller
%%%%%%%%%%%%%%%%%%%%%%%%%%%%%%%%%%%%%%%%
\begin{figure}
    \centering
    \includegraphics[width=1.0\columnwidth]{pics/reconstructed_MNIST/weighted/task_recon_zdim_4_reconstruction_70.png}
    \caption{\textbf{MNIST with reconstruction loss}: Our general co-design framework of \name allows highly-compressible, but also human-interpretable decoded images. Specifically, when we optimize for classification task loss and weighted reconstruction loss, with weight $\lambda=0.01$ (Eq. \ref{eq:weighted_loss}), decoded images $\xhat$ (bottom row) are human-interpretable and resemble original images $x$ (top row). However, the key benefit of \name is that we have a heavily-compressed bottleneck representation of $\zbottleneck=4$, which is much smaller than task-agnostic representations, as shown in Fig. \ref{fig:MNIST_task_recon_loss}. We note that the decoded samples emphasize salient features for machine classification and do not produce the sharpest reconstructions since reconstruction is not the \textit{primary} objective. However, these blurry decoded samples $\xhat$ are sufficient to achieve high \textit{machine} classification accuracy.}
    \label{fig:mars_recon_weighted}
\end{figure}
