# Supplementary material for: Personalized Federated Learning of Driver Prediction Models for Autonomous Driving
Source: arXiv:2112.00956 source file (2021-12-02)
Supplement: Supplementary file 6 [file MNIST_recon_weighted_2.tex]

% smaller
%%%%%%%%%%%%%%%%%%%%%%%%%%%%%%%%%%%%%%%%
\begin{figure}
    \centering
    \includegraphics[width=1.0\columnwidth]{pics/reconstructed_MNIST/weighted/task_recon_zdim_4_reconstruction_60.png}
    \caption{\textbf{MNIST with reconstruction loss}: 
    A further example of how our general co-design framework of \name allows highly-compressible, but also human-interpretable decoded images. This example mirrors Fig. \ref{fig:mars_recon_weighted}, but for another set of data.}
    \label{fig:mars_recon_weighted_2}
\end{figure}
