# Supplementary material for: Personalized Federated Learning of Driver Prediction Models for Autonomous Driving
Source: arXiv:2112.00956 source file (2021-12-02)
Supplement: Supplementary file 7 [file mars_hirise.tex]

% smaller
%%%%%%%%%%%%%%%%%%%%%%%%%%%%%%%%%%%%%%%%
\begin{figure}
    \centering
    \includegraphics[width=1.0\columnwidth]{pics/mars_hirise/task_accuracy_mars_hirise.pdf} % first figure itself
    \caption{\textbf{Mars terrain classification:} This plot illustrates our ability to flexibly allocate compute between a resource-constrained robot and cloud server. Specifically, as described in Sec. \ref{subsec:mars}, we can run layers until EfficientNet block $b$, co-design task relevant encoder/decoder to transmit intermediate computations, and finally continue computation with the rest of the \textit{pre-trained} EfficientNet at a server. We plot \name with $\lambda=0$ for scenarios where the robot only runs up to EfficientNet block $b$ locally and achieve within $1\%$ of the uncompressed input error rate (green dashed line) at block $4c$ and beyond for $\zbottleneck=128$.}
    \label{fig:mars_hirise_all_splits}
\end{figure}
