# Supplementary material for: Personalized Federated Learning of Driver Prediction Models for Autonomous Driving
Source: arXiv:2112.00956 source file (2021-12-02)
Supplement: Supplementary file 8 [file modular_compute.tex]

% smaller
%%%%%%%%%%%%%%%%%%%%%%%%%%%%%%%%%%%%%%%%
\begin{figure}
    \centering
    \includegraphics[width=1.0\columnwidth]{pics/appendix_pics/mars_example.pdf}
    \caption{\textbf{Remote perception configuration:} This figure illustrates the conventional configuration of \name, where the robot's learned encoder maps sensory input $x$ to compressed representation $z$. After $z$ is transmitted over a network link, it is decoded to $\xhat$ at a server and directly passed to a pre-trained, modular task network $\ftask(;\thetatask)$ that fully runs at a remote server. This configuration corresponds to Fig. \ref{fig:task_autoencoder}, which complements the alternative architecture in Fig. \ref{fig:tasknet_architecture} where \name flexibly allocates computation that is split between a robot and server.}
    \label{fig:modular_compute}
\end{figure}
