# Supplementary material for: Personalized Federated Learning of Driver Prediction Models for Autonomous Driving
Source: arXiv:2112.00956 source file (2021-12-02)
Supplement: Supplementary file 9 [file motion_plan_mars_2.tex]

% smaller
%%%%%%%%%%%%%%%%%%%%%%%%%%%%%%%%%%%%%%%%
\begin{figure}
    \centering
    \includegraphics[width=1.0\columnwidth]{pics/MPNET_mars_pictures/terrain_2133_2893_paper.pdf} % first figure itself
    \caption{\textbf{Motion planning on Mars Terrain Data}: A further example of how \name can plan feasible, collision-free motion plans on out-of-domain Mars data, as illustrated in Fig. \ref{fig:mars_generalization} and \ref{fig:mars_motion_plan}.}
    \label{fig:mars_motion_plan_2}
\end{figure}
