# Supplementary material for: Personalized Federated Learning of Driver Prediction Models for Autonomous Driving
Source: arXiv:2112.00956 source file (2021-12-02)
Supplement: Supplementary file 10 [file tasknet_architecture.tex]

% smaller
%%%%%%%%%%%%%%%%%%%%%%%%%%%%%%%%%%%%%%%%
\begin{figure}
    \centering
    \includegraphics[width=1.0\columnwidth]{pics/appendix_pics/tasknet_architecture.pdf} % first figure itself
    \caption{\textbf{Flexible allocations of robot and server compute:} An example configuration for flexibly allocating compute between a robot and server, used for the EfficientNet Mars classification examples in Sec. \ref{subsec:mars}. Specifically, we can take the \textit{pre-trained} EfficientNet and insert a learned, task-relevant encoder to map an intermediate feature map to a bottleneck representation $z$. Once $z$ is transmitted over a wireless link, the learned decoder uncompresses the intermediate feature map so that computation can continue at a remote server with the rest of the pre-trained EfficientNet. Our flexible co-design algorithm also allows the modular EfficientNet to fully run at a remote server.}
    \label{fig:tasknet_architecture}
\end{figure}
