# Supplementary material for: Personalized Federated Learning of Driver Prediction Models for Autonomous Driving
Source: arXiv:2112.00956 source file (2021-12-02)
Supplement: Supplementary file 11 [file appendix.tex]

\begin{comment}

In this section, we provide further experimental results to illustrate the benefits of co-designing sensory representations with a pre-trained task module's objective using our \name algorithm. Specifically, we elaborate on results for:

\begin{enumerate}
    \item linear task-aware compression (Sec. \ref{appendix:linear})
    \item martian terrain classification with EfficientNets (Sec. \ref{appendix:terrain})
    \item neural motion planning (Sec. \ref{appendix:motion_plan})
    \item anomaly detection of environmental sensor timeseries (Sec. \ref{appendix:environmental_sensor}), and
    \item decoding human-interpretable reconstructed sensory inputs (Sec. \ref{appendix:MNIST}).
\end{enumerate}

% linear
%%%%%%%%%%%%%%%%%%%%%%%%%%%%%%%%%%%%%%%%%%%%%%%%
\subsection{Further analysis of Linear Task-aware compression}
\label{appendix:linear}
Consider the linear setting described in Sec. \ref{subsec:linear_setup}, where
the encoder is a matrix $\Aencoder \in \reals^{\zbottleneck \times \ninput}$ and the decoder is also a matrix $\Bdecoder \in \reals^{\ninput \times \zbottleneck}$. Recall that the original sensory input is given by $x \in \reals^\ninput$ and reconstructed sensory input is given by $\hat{x} = BAx$, while the task output is denoted by $y = \KLQR x$. \\


We now consider the weighted loss function with $\lambda > 0$, where
\begin{align*}
    \weightedloss = \Vert (\KLQR x - \KLQR \Bdecoder \Aencoder x) \Vert^2_2 + \lambda \Vert(\reconoperand)\Vert^2_2. \\
\end{align*}

In the linear setting, solving Problem \ref{prob:codesign} for a fixed task matrix $K$ amounts to setting the gradient of the weighted task loss with respect to the encoder and decoder matrices to zero. 
Thus, the optimal encoder/decoder matrices that minimize weighted task loss must satisfy:

\begin{align*}
    \nabla_{\Aencoder} \weightedloss &= -2 \Bdecoder^T \KLQR^T (\taskoperand) x^T \\ & -2 \lambda \Bdecoder^T (\reconoperand) x^T \\
    \nabla_{\Bdecoder} \weightedloss &= -2 \KLQR^T (\taskoperand) x^T \Aencoder^T \\ &- 2 \lambda (\reconoperand) x^T \Aencoder^T 
\end{align*}

If we run our co-design algorithm Alg. \ref{alg:train} and use the \textit{analytical} gradients computed above in the backpropagation step, we arrive at the results in Figs. \ref{fig:LQR_simulation_3D} and \ref{fig:LQR_simulation}. Specifically, we see the task-aware weighted scheme achieves the upper bound task accuracy with low reconstruction loss for $\zbottleneck \ge \text{rank}(K)$. Further, the relative merits of our weighted task-aware scheme mirror the trends shown in the large-scale deep learning experiments.

\input{figure_latex/appendix/LQR.tex}

% classification
%%%%%%%%%%%%%%%%%%%%%%%%%%%%%%%%%%%%%%%%%%%%%%%%
\subsection{Further Description of Mars Terrain Classification with EfficientNet}
\label{appendix:terrain}
In Sec. \ref{subsec:mars}, we showed how to flexibly allocate compute resources between a resource-constrained robot and server for terrain classification with EfficientNets. Fig. \ref{fig:mars_hirise_labels} illustrates the training data from the HiRise dataset \cite{hirise}. Then, Fig. \ref{fig:tasknet_architecture} illustrates how we can flexibly allocate compute between a small robot and server with the \name architecture. However, we emphasize that our design also allows the full, modular EfficientNet task network to be run remotely, as depicted in the complementary configuration in Fig. \ref{fig:modular_compute}. Finally, Fig. \ref{fig:mars_hirise_all_splits} illustrates the resultant classification task accuracy for various configurations of computation allocated between a robot and server.

\input{figure_latex/appendix/example_mars_labels.tex}
\input{figure_latex/appendix/tasknet_architecture.tex}
\input{figure_latex/appendix/modular_compute.tex}
\input{figure_latex/appendix/mars_hirise.tex}

% motion planning
%%%%%%%%%%%%%%%%%%%%%%%%%%%%%%%%%%%%%%%%%%%%%%%%
\subsection{Generalization of Neural Motion Planning to out-of-domain Mars Data}
\label{appendix:motion_plan}
In Section \ref{subsec:motion_planning} and Figs. \ref{fig:mars_generalization} and \ref{fig:mars_motion_plan}, we showed that \name generalizes to never-before-seen Mars terrain data, where obstacle point clouds have significantly different shapes than those of the \MPNET training and test data. Further examples of the \name co-designed motion planner are provided in Fig. \ref{fig:mars_motion_plan_2}.

\input{figure_latex/appendix/motion_plan_mars_2.tex}


%%%%%%%%%%%%%%%%%%%%%%%%%%%%%%%%%%%%%%%%%%%%%%%%
\subsection{Further Description of Environmental Sensor Experiments}
\label{appendix:environmental_sensor}

Fig. \ref{fig:IoT} shows example timeseries that we collected from an environmental sensor board connected to the Edge TPU DNN accelerator. Our comprehensive dataset spans two weeks of diverse, stochastic timeseries described in Sec. \ref{subsec:IoT}.

\input{figure_latex/appendix/IOT_TPU.tex}

\subsection{Effects of reconstruction loss on decoded images}
\label{appendix:MNIST}
In Eq. \ref{eq:weighted_loss}, we allow a roboticist to optimize for task loss, but also optionally for reconstruction loss, in scenarios where decoded inputs $\xhat$ need to be sanity-checked or viewed remotely to debug. For the MNIST experiments in Sec. \ref{subsec:MNIST}, we show how introducing a reconstruction loss weight $\lambda > 0$ yields highly-compressible, but human-interpretable results in Figs. \ref{fig:mars_recon_weighted} and \ref{fig:mars_recon_weighted_2}. We contrast these with the case where we optimize \textit{solely} for a machine's task loss in Figs. \ref{fig:mars_recon_unweighted} and \ref{fig:mars_recon_unweighted_2} with $\lambda=0$.

\label{appendix:MNIST_recon}
\input{figure_latex/appendix/MNIST_recon_weighted.tex}
\input{figure_latex/appendix/MNIST_recon_unweighted.tex}

\input{figure_latex/appendix/MNIST_recon_weighted_2.tex}
\input{figure_latex/appendix/MNIST_recon_unweighted_2.tex}

\end{comment}
